# Supplementary material for: Reciprocal Multi-Robot Collision Avoidance with Asymmetric State Uncertainty
Source: arXiv:2107.10956 source file (2021-07-22)
Supplement: Supplementary file 1 [file 7_appendix.tex]

% \section{Appendix}
% \subsection{Dual functions}
% In this subsection, we derive the Lagrange dual function for the Voronoi cell
% generated by polyhedra.

% \paragraph{Polyhedra.}
% In the case where our set $\ellipse$ is specified by an affine constraint (\ie,
% $\ellipse$ is a polyhedron),
% \[
% \ellipse = \{y ~|~ Ay \le b\},
% \]
% with $A \in \reals^{m\times n}$ and $b \in \reals^m$, then the dual function can be easily computed.

% First, note that the minimizer of $\normsq{y} - 2c^Ty$ can be found by setting the gradient to zero (this is necessary and sufficient by convexity and differentiability), which yields that the optimal point is $y^* = c$, with optimal value
% \[
% \inf_y\left(\normsq{y} + 2c^Ty\right) = -\normsq{c}.
% \]
% Applying this result yields
% \[
% g(x, \lambda) = \inf_y \left(\normsq{y} - 2x^Ty + \lambda^T(Ay - b)\right) = - \normsq{x-A^T\lambda/2} - b^T\lambda,
% \]
% with $\lambda \ge 0$.

% \subsection{Extensions}
% There are several natural extensions to problem~(\ref{eq:main}). These extensions can be combined, as needed.

% \paragraph{Union of convex sets.} We can extend the formalism of~(\ref{eq:main}) to include the Voronoi region generated by a finite union of convex sets. That is, if $S$ can be written in the form
% \[
% S = \bigcup_{i=1}^\ell ~\{y~|~f_i(y) \le 0\},
% \]
% for convex functions $f_i: \reals^n \to \reals^{m_i}$. Note that, in general,
% $S$ will not be convex, while the resulting Voronoi region always is, since the
% region is the intersection of a family of hyperplanes. Additionally, we will
% require that there exist $y_i^0\in \reals^n$ with $f_i(y_i^0) < 0$ for $i=1,
% \dots, \ell$ if $f_i$ is not affine. The corresponding problem is given by
% \[
% \begin{array}{ll}
% \mbox{minimize}   & \normsq{x - \xgoal} \\
% \mbox{subject to} & \normsq{\xcurr} - 2x^T\xcurr \le \inf_{f_i(y) \le 0} \left(\normsq{y} - 2y^Tx\right), ~~ i=1, \dots, \ell.
% \end{array}
% \]
% In this case, we simply derive a dual function for each constraint with $i=1, \dots, \ell$, writing each as a constraint as in~(\ref{eq:dual-form}), each of which is convex.

% \paragraph{Intersection of a convex set with the Voronoi cell.}
% Given a convex set $C$ specified by
% \[
% C = \{x ~|~ h(x) \le 0\},
% \]
% where $h:\reals^n \to \reals^r$ is a convex function, then the problem
% \[
% \begin{array}{ll}
% \mbox{minimize}   & \normsq{x - \xgoal} \\
% \mbox{subject to} & \normsq{\xcurr} - 2x^T\xcurr \le \inf_{f(y) \le 0} \left(\normsq{y} - 2y^Tx\right)\\
% & h(x) \le 0,
% \end{array}
% \]
% is the intersection of the Voronoi cell in question and the set $C$, which is also easily solvable assuming $h$ can be easily evaluated at any point in its domain.
